# Supplementary material for: Multi-axis inertial sensing with long-time point source atom interferometry
Source: arXiv:1305.1700 ancillary file (2013-05-08)
Supplement: Supplementary file 1 [file SupplementalMaterial.pdf]

# Supplemental Materials: Multi-axis inertial sensing with long-time point source atom interferometry

Susannah M. Dickerson, Jason M. Hogan, Alex Sugarbaker, David M. S. Johnson, and Mark A. Kasevich
*Department of Physics, Stanford University, Stanford, California 94305*

## PRINCIPAL COMPONENT ANALYSIS

Principal Component Analysis (PCA) is a statistical analysis procedure that can identify correlations within a data set in a model-independent way [1]. When applied to a set of images, the result is a basis of orthonormal image vectors that spans the initial image set. These basis image vectors are called the principle components, and they are typically ordered by their variance. The higher the variance, or 'strength,' the better the basis image accounts for the variability of the set of images as a whole. By projecting a particular image in the original set onto a subspace of the principal component basis, we can isolate different correlations of interest from other correlations or backgrounds [1, 2].

Since interference is an anti-correlation between atom populations between output ports and (in the case of spatially-dependent phase) between neighboring slices within an output port, we can use PCA to distinguish between the constant overall shape of the ports, the interfering atom populations, and sources of technical noise (e.g. camera electronic noise) and systematic noise (e.g. launch velocity or cloud shape jitter).

In Fig. 1 we show the first six of 20 principal components for a set of 20 images. For this set, a rotation of $40\,\mu$rad/s was applied in excess of what was required for rotation compensation. The lower (unpushed) port of the second principal component is also displayed in Fig. 2 of the main text. The first component shows the features most common in all the images of the set: the overall envelope of the two output ports. The next pair of principal components are the two quadratures of the fringe (sine and cosine). Both quadratures emerge as principal components because the input image set consists of images with widely varying overall interferometer phase (the phase is scanned randomly over multiple radians due to the vibrations of the retroreflection mirror). Any possible interferometer phase can be represented by a weighted sum of these two principal components. Note that given an infinite number of images with uniformly distributed phase, the variance of these two components should be identical; this is not the case for the specific finite data set used for Fig. 1 because in this set (by chance) there are more "sine-like" images that "cosine-like" images. Alternatively, given a set of images with a fixed interferometer phase (i.e., no vibration noise), the spatial fringes would appear on the first principal component as a common feature of all the images. Notice that a $\pi$ phase shift between the two output ports of a single principal component is clearly visible in these images, a signature of interference. The depth of the fringes in the upper port is reduced due to heating from the optical push used to spatially separate the output ports.

PCA can be used as a filter by projecting each image into a subspace spanned by the strongest principal components. The projection onto the first three components (cloud shape, sine fringe, and cosine fringe) typically shows greater than 99% overlap with the original image. The higher principal components may nevertheless contain valuable information. The fourth component in Fig. 1, for example, shows a common-mode vertical correlation between the two output ports, indicative of a jitter in the vertical launch velocity of the initial cloud. For higher principal components, however, the spatial frequencies tend to increase until the basis images appear to consist of high-frequency noise (not shown).

We take advantage of the linearity of PCA to robustly estimate the fringe contrast. We project each image in the set both onto (1) the overall cloud envelope (principal component 1) and separately onto (2) the subspace of the cosine and sine quadratures (principal components 2 and 3). We then independently fit these two projections for the un-pushed port, binned vertically to reduce dimensionality. The contrast is then given by the ratio of the amplitudes of those two fits. Fitting the fringe and the envelope separately increases the robustness of the fit by reducing cross-talk between fitting parameters.

We model the general shape of the upper $(P_U(x,z))$ and lower $(P_L(x,z))$ output ports as Gaussians in two dimensions (we have already integrated over the third dimension in the creation of the 2D image). The expected population distribution within each cloud depends on the interferometer phase, which we allow to vary transversely with $x$: $\Delta\phi(x) = k_x x + \phi$. If the clouds are well-separated, we can integrate (bin) over the vertical dimension, leaving to good approximation

$$P_U(x) = A_U e^{-\frac{x^2}{2\sigma_x^2}} \left(\frac{1}{2} + \frac{c}{2}\sin\left[k_x x + \phi\right]\right) \qquad (1)$$

$$P_L(x) = A_L e^{-\frac{x^2}{2\sigma_x^2}} \left(\frac{1}{2} - \frac{c}{2}\sin\left[k_x x + \phi\right]\right) \qquad (2)$$

The two output ports differ only by a $\pi$ phase shift. When we use PCA, we fit each of the two terms in an output port separately. Considering just one port, the

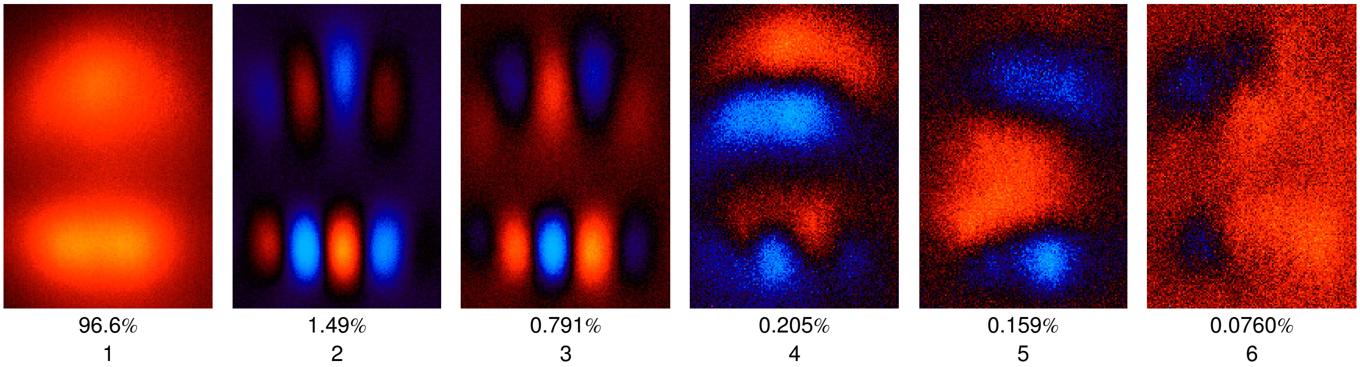


FIG. 1. Normalized principal components, numbered according to their mean percentage overlap with the original images. These normalized basis images are colored to identify regions of correlation (same color) and anticorrelation (blue versus red). The upper port has been heated by the push used to spatially separate the two ports, resulting in a reduction of the contrast of the fringes in that port.

population in that port is modeled as

$$P_L\left(x\right) = P_1\left(x\right) + P_{\text{fringe}}\left(x\right) \tag{3}$$

$$P_1\left(x\right) = A_1 e^{-\frac{x^2}{2\sigma_x^2}} \tag{4}$$

$$P_{\text{fringe}}\left(x\right) = -A_{\text{fringe}} e^{-\frac{x^2}{2\sigma_x^2}} \sin\left[k_x x + \phi\right] \tag{5}$$

We then independently fit Eqs. 4 and 5 to the envelope and fringe projections, respectively. Comparing Eq. 3 to Eq. 2 we see that the contrast $c$ can be recovered by $A_{\text{fringe}}/A_1$, the ratio of the amplitude of the fringe to the amplitude of the envelope. The fit to the spatial frequency of the fringe, $k_x$, is a direct measurement of the phase gradient.

When the wavelength of the fringe is long compared to the cloud size, a fit to the fringe of a single output port cannot accurately determine the spatial frequency and the phase, leading to a mischaracterization of fringe amplitude and the contrast. In this small-gradient regime, ellipse analysis can provide more accurate information about the phase gradient.

[1] S. R. Segal, Q. Diot, E. A. Cornell, A. A. Zozulya, and D. Z. Anderson, Physical Review A **81**, 053601 (2010).
[2] S.-w. Chiow, T. Kovachy, H.-C. Chien, and M. A. Kasevich, Physical Review Letters **107**, 130403 (2011).
